# Supplementary material for: Improving Feature Stability during Upsampling -- Spectral Artifacts and the Importance of Spatial Context
Source: arXiv:2311.17524 source file (2024-07-12)
Supplement: Supplementary file 1 [file boat_comparing_predictions.tex]

\begin{figure*}[t]
     \centering
     \begin{subfigure}[b]{0.3\textwidth}
         \centering
         \includegraphics[width=\textwidth]{cvpr2023-author_kit-v1_1-1/figures/appendix/segmentation/feature_maps/gt_2007_000061.png}
         \caption{Ground truth segmentation mask of the third image in the test set.\newline}
         \label{fig:appendix:exp:segmentation:boat:gt}
     \end{subfigure}
     \hfill
     \begin{subfigure}[b]{0.3\textwidth}
         \centering
         \includegraphics[width=\textwidth]{cvpr2023-author_kit-v1_1-1/figures/appendix/segmentation/feature_maps/trans_2_vanilla_backbone_2007_000061.png}
         \caption{Baseline: using 2 x 2 kernel sizes in transposed convolution layers and 3 x 3 convolution kernels in the decoder blocks}
         \label{fig:appendix:exp:segmentation:boat:baseline_pred}
     \end{subfigure}
     \hfill
     \begin{subfigure}[b]{0.3\textwidth}
         \centering
         \includegraphics[width=\textwidth]{cvpr2023-author_kit-v1_1-1/figures/appendix/segmentation/feature_maps/trans_11_3_vanilla_backbone_2007_000061.png}
         \caption{Using 11 x 11 + 3 x 3 kernel sizes in transposed convolution layers and 3 x 3 convolution kernels in the decoder blocks}
         \label{fig:appendix:exp:segmentation:boat:trans11_decoder_conv_3_pred}
     \end{subfigure}
        \caption{Here we compare the predictions from model with large transposed convolution kernels to the baseline, with the same encoder and same convolution blocks in the decoder and also to the ground truth. 
        This is the third test image and an interesting case due to the thin mast in the boat as seen in \cref{fig:appendix:exp:segmentation:boat:gt}. 
        We observe in \cref{fig:appendix:exp:segmentation:boat:baseline_pred} that due to existing grid artifacts, the baseline model is not able to find the mast pixels at all whereas due to large transposed convolution kernels used by the model depicted in \cref{fig:appendix:exp:segmentation:boat:trans11_decoder_conv_3_pred}, it is successfully able to classify some pixel.
        There are also other grid artifacts present in \cref{fig:appendix:exp:segmentation:boat:baseline_pred} which are inhibiting it from predicting a smoother segmentation mask, while the segmentation mask in \cref{fig:appendix:exp:segmentation:boat:trans11_decoder_conv_3_pred} is better able to match the shape of the boat and thus the ground truth.}
        \label{fig:appendix:experiments:segmentation:boat:comparing_predictions}
\end{figure*}
