# Supplementary material for: Improving Feature Stability during Upsampling -- Spectral Artifacts and the Importance of Spatial Context
Source: arXiv:2311.17524 source file (2024-07-12)
Supplement: Supplementary file 2 [file freq_comparison.tex]

\begin{figure}[t]
	\begin{center}
	\includegraphics[width=1.0\linewidth]{cvpr2023-author_kit-v1_1-1/figures/appendix/disparity/with_9_loglog_freq_comparison_norm.pdf}
	\caption[]{Comparison of feature maps from the penultimate layer of the ``feature extractor" in STTR-light\cite{sttr}. 
	Unlike \cref{fig:intro:teaser}, in this downstream task, the ground truth is not a segmentation mask but disparity estimation, thus a ground truth whose property the feature maps intend to mimic is not available for comparison.
	Thus, we compare to the input images in the frequency domain. ``Left" are the features and input from the left frame, similarly ``Right" indicated the right frame.
	Since ``FlyingThings3D"\cite{flyingthings_MIFDB16} is a synthetic dataset, the frequencies in the input images are not smooth and have some oscillations.
	These oscillations are reflected in the feature maps.
	The feature maps from the small (3$\times$3) kernel for transposed convolution for upsampling(baseline) shows the most power in the oscillations and thus the poor performance.
	As the size of the kernel is increased to 7$\times$7, the power of the peaks and the oscillations reduces, thus leading to better performance, as similar to as discussed in \cref{subsec:exp:semantic} this indicates that the network is learning better upsampling.
	However, in this case, as the size of the kernels are increased further, or a small kernel is added in parallel, we observe that the power of the peaks reduces only slightly.
	Moreover, in the high frequency region, the power of the frequencies even slightly surpass those of the baseline.
	Thus indicating a limit of the size of the kernels for this downstream task.
	This is indicated in the empirical performance of these design choices as well.}
	\label{fig:appendix:disparity:freq_comparison}
	\end{center}
\end{figure}
