# Supplementary material for: Improving Feature Stability during Upsampling -- Spectral Artifacts and the Importance of Spatial Context
Source: arXiv:2311.17524 source file (2024-07-12)
Supplement: Supplementary file 3 [file baseline_aeroplane.tex]

\begin{figure*}[t]
	\begin{center}
	\includegraphics[width=1.0\textwidth]{cvpr2023-author_kit-v1_1-1/figures/appendix/segmentation/feature_maps/marked_trans_2_vanilla_backbone_2007_000033_binary_map.pdf}
	\caption[]{Full feature map from the first test image in the validation dataset for the baseline model.
	Channels marked with red arrow and circled were the ones used in the \cref{fig:exp:segmentation:comparing_pred_features}}
	\label{fig:appendix:segmentation:feature:baseline:aeroplane}
	\end{center}
\end{figure*}
