# Supplementary material for: Improving Feature Stability during Upsampling -- Spectral Artifacts and the Importance of Spatial Context
Source: arXiv:2311.17524 source file (2024-07-12)
Supplement: Supplementary file 4 [file comparing_fgsm_freq.tex]

\begin{figure*}[t]
	\begin{center}
	\includegraphics[width=1.0\textwidth]{cvpr2023-author_kit-v1_1-1/figures/appendix/segmentation/fgsm_freq/unet_fgsm_convnext_comparison_zoomed.pdf}
	\caption[]{Comparing frequency spectra from different architectural choices caused by varying intensities of FGSM attack, averaged over 725 test samples. The region bounded in the red box is shown in the zoomed window above it. `epsilon 0.0' denotes input images with no perturbations by FGSM attack, i.e. clean images.}
	\label{fig:appendix:segmentation:comparing_fgsm_freq}
	\end{center}
\end{figure*}
