# Supplementary material for: Improving Feature Stability during Upsampling -- Spectral Artifacts and the Importance of Spatial Context
Source: arXiv:2311.17524 source file (2024-07-12)
Supplement: Supplementary file 5 [file frequency_spectra_image_mask.tex]

\begin{figure}[t]
     \centering
     \begin{subfigure}[b]{0.85\linewidth}
         \centering
         \includegraphics[width=\linewidth]{cvpr2023-author_kit-v1_1-1/figures/appendix/freq_diff_real_world/real_world_vs_ground_truth_top_legend.pdf}
         \caption{Frequency spectra of Real world and Segmentation masks.}
         \label{fig:appendix:real_world}
     \end{subfigure}
     \vfill
     \begin{subfigure}[b]{0.85\linewidth}
         \centering
         \includegraphics[width=\linewidth]{cvpr2023-author_kit-v1_1-1/figures/appendix/freq_diff_real_world/fgsm_input_vs_ground_truth_top_legend.pdf}
         \caption{Change in frequency spectra due to FGSM attack.}
         \label{fig:appendix:real_world_fgsm_variation}
     \end{subfigure}
        \caption{A comparison of the frequency spectra of real world input images and segmentation masks in PASCAL VOC 2012 validation dataset. \cref{fig:appendix:real_world} shows us that the segmentation mask has many oscillating frequencies, especially in the high frequency range, whereas the real world data is more or less smooth having very different frequency properties than the segmentation mask. In \cref{fig:appendix:real_world_fgsm_variation} we observe the change in frequency profile caused due to perturbations in the images using FGSM attack.}
        \label{fig:appendix:real_world_and_fgsm}
        \vspace{-1em}
\end{figure}
