# Supplementary material for: Improving Feature Stability during Upsampling -- Spectral Artifacts and the Importance of Spatial Context
Source: arXiv:2311.17524 source file (2024-07-12)
Supplement: Supplementary file 6 [file interpolation_freq.tex]

\begin{figure}[t]
	\begin{center}
	\includegraphics[width=\linewidth]{cvpr2023-author_kit-v1_1-1/figures/appendix/pspnet/vanilla_pspnet_resnset50_freq_473.pdf}
	\caption[]{Comparing frequency spectra of feature maps of the penultimate layer in PSPNet with ResNet50 backbone to the ground truth. Since authors use a 473$\times$473 sized sliding window for training and testing, the ground truth(left) and feature maps(right) are from the last 473$\times$473 crop of the target and input respectively. Here we clearly observe that PSPNet has smoothened out almost all the frequencies.}
	\label{fig:appendix:interpolation:freq}
	\end{center}
\end{figure}
