# Supplementary material for: Improving Feature Stability during Upsampling -- Spectral Artifacts and the Importance of Spatial Context
Source: arXiv:2311.17524 source file (2024-07-12)
Supplement: Supplementary file 7 [file kernel_limit.tex]

\begin{figure}[t]
	\begin{center}
	\includegraphics[width=1.0\linewidth]{cvpr2023-author_kit-v1_1-1/figures/appendix/limit_31/botton_legend_limit_test_31_11_comparison.pdf}
	\caption[]{Comparison of feature maps from the penultimate layer, similar to \cref{fig:intro:teaser} except the size of the transposed convolution kernel, entire architecture is the same with the 3$\times$3 kernels for convolution layers in the decoder building block.
	We observe that 31$\times$31 + 3$\times$3 kernels are introducing a new peak, adding to the spectral artifacts and thus performing poorly. 
	Moreover, both 31$\times$31 + 3$\times$3 and 31$\times$31 + 5$\times$5 are not suppressing the power of the peaks of the oscillation when compared to 11$\times$11 + 3$\times$3, thus further explaining their lower performance.}
	\label{fig:appendix:kernel_limit}
	\end{center}
\end{figure}
