# Supplementary material for: Improving Feature Stability during Upsampling -- Spectral Artifacts and the Importance of Spatial Context
Source: arXiv:2311.17524 source file (2024-07-12)
Supplement: Supplementary file 8 [file parallel_kernel_fgsm.tex]

\begin{figure}[t]
	\begin{center}
	\includegraphics[width=1.0\linewidth]{cvpr2023-author_kit-v1_1-1/figures/appendix/parallel_kernel/window_fgsm_trans_0_comparison.pdf}
	\caption[]{A comparison of feature maps in frequency domain when using and not using small parallel kernel in transposed convolution for upsampling.
	Both architectures have the same 3$\times$3 convolutions in the decoder block.
	As discussed in \cref{subsec:exp:semantic}, transposed convolution with 11$\times$11 + 3$\times$3 kernels is able to suppress power of oscillations to a greater extent than other kernel sizes. (Right) Transposed convolution with no 3$\times$3 parallel kernel is not able to suppress the power of oscillations(compared to left), especially as the intensity of FGSM attack increases.
	This shows that it is not learning as good upsampling. 
	Thus, resulting in comparatively poor performance against adversarial attacks.}
	\label{fig:appendix:parallel_kernel_fgsm}
	\end{center}
\end{figure}
