# Supplementary material for: Improving Feature Stability during Upsampling -- Spectral Artifacts and the Importance of Spatial Context
Source: arXiv:2311.17524 source file (2024-07-12)
Supplement: Supplementary file 9 [file prediction_difference.tex]

\begin{figure*}[t]
	\begin{center}
	\includegraphics[width=1.0\textwidth]{cvpr2023-author_kit-v1_1-1/figures/appendix/segmentation/predictions/prediction difference.pdf}
	\caption[]{A comparison of predictions for the shown input images and ground truth segmentation masks. The row labelled ``Prediction Difference" shows the difference in predictions among the ground truth, baseline model's predictions and predictions from model similar to baseline except with 11$\times$11 (+3$\times$3) kernels in transposed convolution(comparison model). White pixel is where both baseline and comparison models had correct predictions(same as ground truth). Red pixel is where baseline model predicted correctly but comparison model predicted incorrectly. Green pixel is where the comparison model predicted correctly but the baseline model predicted incorrectly. Black pixel is where both baseline and comparison models predicted incorrectly.}
	\label{fig:appendix:segmentation:prediction_difference}
	\end{center}
\end{figure*}
