# Supplementary material for: Improving Feature Stability during Upsampling -- Spectral Artifacts and the Importance of Spatial Context
Source: arXiv:2311.17524 source file (2024-07-12)
Supplement: Supplementary file 10 [file trans_11_3_aeroplane.tex]

\begin{figure*}[t]
	\begin{center}
	\includegraphics[width=1.0\textwidth]{cvpr2023-author_kit-v1_1-1/figures/appendix/segmentation/feature_maps/marked_trans_11_3_vanilla_backbone_2007_000033_binary_map.pdf}
	\caption[]{Full feature map from the first test image in the validation dataset for the segmentation model with 11$\times$11 kernels in transposed convolution for upsampling and ResNet-style backbone with 3$\times$3 kernels in the convolution layers of the decoder building blocks. Channels marked with red arrows were the ones used in the \cref{fig:exp:segmentation:comparing_pred_features}}
	\label{fig:appendix:segmentation:feature:trans_11_3:aeroplane}
	\end{center}
\end{figure*}

A comparison of final predicted segmentation masks in shown in \Cref{fig:appendix:segmentation:prediction_difference}. We observe that the model with 11$\times$11 (+ 3$\times$3) kernels for transposed convolution is predicting more accurately than the baseline model (2$\times$2 kernels in transposed convolution). This accentuates along corners and areas with sharp edges, where pixels were inaccurately predicted by the baseline due to grid artifacts.
